# Supplementary material for: Symmetry Breaking in Neural Network Optimization: Insights from Input Dimension Expansion
Source: arXiv:2409.06402 source file (2024-09-12)
Supplement: Supplementary file 1 [file suppli.tex]

\documentclass[pdflatex,sn-mathphys-num]{sn-jnl}% Math and Physical Sciences Numbered Reference Style 

%%%% Standard Packages
\usepackage{graphicx}%
\usepackage{multirow}%
\usepackage{amsmath,amssymb,amsfonts}%
\usepackage{amsthm}%
\usepackage{mathrsfs}%
\usepackage[title]{appendix}%
\usepackage{xcolor}%
\usepackage{textcomp}%
\usepackage{manyfoot}%
\usepackage{booktabs}%
\usepackage{algorithm}%
\usepackage{algorithmicx}%
\usepackage{algpseudocode}%
\usepackage{listings}%
\usepackage{adjustbox}
\usepackage{subfigure}

%%%%%=============================================================================%%%%
%%%%  Remarks: This template is provided to aid authors with the preparation
%%%%  of original research articles intended for submission to journals published 
%%%%  by Springer Nature. The guidance has been prepared in partnership with 
%%%%  production teams to conform to Springer Nature technical requirements. 
%%%%  Editorial and presentation requirements differ among journal portfolios and 
%%%%  research disciplines. You may find sections in this template are irrelevant 
%%%%  to your work and are empowered to omit any such section if allowed by the 
%%%%  journal you intend to submit to. The submission guidelines and policies 
%%%%  of the journal take precedence. A detailed User Manual is available in the 
%%%%  template package for technical guidance.
%%%%%=============================================================================%%%%

%% as per the requirement new theorem styles can be included as shown below
\theoremstyle{thmstyleone}%
%  meant for continuous numbers
%%\newtheorem{theorem}{Theorem}[section]% meant for sectionwise numbers
%% optional argument [theorem] produces theorem numbering sequence instead of independent numbers for Proposition
% 
%%\newtheorem{proposition}{Proposition}% to get separate numbers for theorem and proposition etc.

\theoremstyle{thmstyletwo}%

\theoremstyle{thmstylethree}%

\raggedbottom
%%\unnumbered% uncomment this for unnumbered level heads

\begin{document}

\title{Supplementary Information}

\maketitle

The supplementary information contains:
\begin{itemize}
    \item Experimental procedures
    \item Human evaluations
    \item Comparison of GPT4 and ChemCrow for synthesis
    \item Safety workflow
    \item Reproducibility
    \item Limitations
    \item Detailed tasks and evaluations.
\end{itemize}

\maketitle

\newpage

\begin{appendices}

\section{Ablation Study about Expanding Factor}\label{secA}
To further investigate the impact of the expansion factor on image classification performance, we evaluated several models with varying expansion multiples on the CIFAR-10 and CIFAR-100 datasets. As illustrated in Table~\ref{tab-expanding-factor}, image expansion consistently outperforms the direct input of original images into the neural network, regardless of the expansion multiple. Moreover, as the expansion multiple increases, image classification performance generally improves. This improvement can be attributed to the principle of symmetry breaking; increasing the expansion multiple enhances the symmetry of the image, thereby boosting classification performance. These findings further validate the principle of symmetry breaking.

However, indiscriminately increasing the expansion factor can sometimes lead to performance degradation. Our results indicate that the expansion factor should not exceed the size of the kernel in the first convolutional layer of the CNN. Exceeding this limit causes the convolutional kernel to process placeholder data filled during expansion rather than the meaningful original data, leading to a significant drop in performance. This observation supports our earlier assertion that inappropriate symmetry can negatively impact neural network performance.

\begin{table*}[h]
\centering
\caption{Image classification accuracy for CIFAR-10 and CIFAR-100 with various expanding factor. The expansion factor `/' indicates that the image is not expanded.}
\resizebox{0.8\columnwidth}{!}{
\begin{tabular}{c|c|c|c}
\hline
\toprule
Dataset & Model & Expanding & Accuracy (\%) \\
\hline
\multirow{18}{*}{CIFAR-10} & \multirow{5}{*}{ResNet-18} & / & 90.16 \\ \cline{3-4} 
& & 2 & 94.03 \\\cline{3-4} 
& & 3 & 94.61 \\\cline{3-4} 
& & 4 & 94.74 \\\cline{3-4} 
& & 5 & 94.66 \\\cline{2-4} 
 & \multirow{4}{*}{ResNet-50} & / & 86.19 \\\cline{3-4}
& & 2 & 92.14 \\\cline{3-4}
& & 3 & 93.22 \\\cline{3-4}
& & 4 & 94.39 \\\cline{2-4}

 & \multirow{3}{*}{DenseNet-121} & / & 88.72 \\\cline{3-4}
& & 2 & 93.68\\\cline{3-4}
& & 3 & 94.11\\ \cline{2-4}

 & \multirow{3}{*}{MobileNet-v3} & / & 80.92 \\\cline{3-4}
& & 2 & 87.39\\\cline{3-4}
& & 3 & 89.05\\ \cline{2-4}

 & \multirow{3}{*}{EfficientNet} & / & 87.67 \\\cline{3-4}
& & 2 & 91.73\\\cline{3-4}
& & 3 & 92.44\\ \bottomrule

\multirow{18}{*}{CIFAR-100} & \multirow{5}{*}{ResNet-18} & / & 64.28 \\ \cline{3-4} 
& & 2 & 74.70 \\\cline{3-4} 
& & 3 & 76.36 \\\cline{3-4} 
& & 4 & 77.55 \\\cline{3-4} 
& & 5 & 77.02 \\\cline{2-4} 
 & \multirow{4}{*}{ResNet-50} & / & 54.92 \\\cline{3-4}
& & 2 & 70.13 \\\cline{3-4}
& & 3 & 80.28 \\\cline{3-4}
& & 4 & 73.02 \\\cline{2-4}

 & \multirow{3}{*}{DenseNet-121} & / & 62.54 \\\cline{3-4}
& & 2 & 73.14\\\cline{3-4}
& & 3 & 75.41\\ \cline{2-4}

 & \multirow{3}{*}{MobileNet-v3} & / & 50.91 \\\cline{3-4}
& & 2 & 62.63\\\cline{3-4}
& & 3 & 63.36\\ \cline{2-4}

 & \multirow{3}{*}{EfficientNet} & / & 59.45 \\\cline{3-4}
& & 2 & 69.90\\\cline{3-4}
& & 3 & 71.02\\ \bottomrule

\end{tabular}}
\label{tab-expanding-factor}
\end{table*}

\section{Ablation Study about Expanding Filling}\label{secB}
To further investigate the impact of padding values at positions that do not correspond to the original image pixels on image classification, we tested various padding values using the ResNet-18 model on the CIFAR-10 and CIFAR-100 datasets. As shown in Table~\ref{tab-filling}, image expansion enhances classification performance regardless of the padding value used. Notably, even when the padding values are random numbers from a normal distribution—traditionally expected to reduce the signal-to-noise ratio—this approach still improves classification performance. This finding demonstrates that the performance gains from image expansion are not simply due to increased image data, as would be the case with direct interpolation. Instead, the improvement stems from the principle of symmetry breaking. The use of randomly generated values from a normal distribution can enhance performance because, in a statistical sense, it increases the symmetry of the image, aligning with the symmetry-breaking principle.

\begin{table*}[h]
\centering
\caption{Image classification accuracy for CIFAR-10 and CIFAR-100 with various expanding filling with ResNet-18. The term "expansion and filling" refers to the process where, after an image is expanded, certain pixels do not correspond to values from the original image and therefore require placeholder values. Different techniques for filling these placeholders are evaluated to determine their impact on classification accuracy, where `Random' represents the values of padding elements at different positions in the expanded image is a normally distributed stochastic number.}
\resizebox{0.6\columnwidth}{!}{
\begin{tabular}{c|c|c}

\hline
\toprule
Dataset &  Filling & Accuracy (\%) \\ \hline
\multirow{5}{*}{CIFAR-10} &  0.0  & 94.74 \\ \cline{2-3} 
&  0.25 & 92.86 \\\cline{2-3} 
&  0.50 & 92.30 \\\cline{2-3} 
&  1.0 & 92.60 \\\cline{2-3} 
&  Random & 91.56 \\ \bottomrule 

\multirow{5}{*}{CIFAR-100} &  0.0  & 68.48 \\ \cline{2-3} 
&  0.25 & 68.91 \\\cline{2-3} 
&  0.50 & 68.99 \\\cline{2-3} 
&  1.0 & 69.11 \\\cline{2-3} 
&  Random & 66.39 \\ \bottomrule 

\end{tabular}
}
\label{tab-filling}
\end{table*}

\end{appendices}

\end{document}
